# Supplementary material for: Automatic Generation of Personalized Comment Based on User Profile
Source: arXiv:1907.10371 source file (2019-07-24)
Supplement: Supplementary file 2 [file SupplementrayMaterial.pdf]

# Supplementary Materials for the ACL Student Research Workshop Submission: Automatic Generation of Personalized Comment

April 25, 2019

## 1 Case Study

We present some examples in Figure 2, 3. As can be seen, for a given blog, there are multiple users (users profile are shown in Figure 1) that are suitable for its response in comments. Seq2Seq generates a comment with a random user. PCGN can generate personalized comment conditioned on given user. According to the user profile, user 1 is more adores Yilong Zhu[1], So for the blogs related to Yilong Zhu , user 1 tend to express their affection in comments. For some users, their individual description can not offer helpful information or there is missing value for individual description. In this case, the PCGN model pay more attention to numeric features and learned representation from similar seen users.

| User | Age | Birthday | Gender | Province | City | Individual Description |
|---|---|---|---|---|---|---|
| U1 | 24 | 1994-5-20 | 女<br>Female | 其他<br>Others | NULL | 只爱朱一龙<br>I only love Yilong Zhu |
| U2 | 23 | 1995-4-28 | 女<br>Female | 黑龙江<br>Heilong Jiang | NULL | 努力成为更好的自己<br>Become a better me |
| U3 | 20 | 1998-3-06 | 女<br>Female | 浙江<br>Zhejiang | 宁波<br>Ningbo | NULL |

Figure 1: Part of user profile of case study users.

[1]A famous Chinese star

| **Blog** |
| --- |
| # 朱一龙 温柔的力量 [ 超话 ] # [ 小仙女 ] # 朱一龙并肩前行 # 遇见你，是旷野的风闯进心房，是眉间的闯进眼眶。想把一切与你分享，清晨的暖阳、浩瀚的夜空、过去的美好、 未来的相伴。「朱一龙」<br>Yilong Zhu Gentle power [super topic]# walking side by side with Yilong Zhu#The moment I met you seems like the wind of the wilderness, breaking into my heart. The moment I met you seems like the snow between the eyebrows, blending into the eyes. I want to share everything with you, the warm sun in the morning, the vast night sky, the beauty of the past and the companion in the future. |
| **Comments** |
| Seq2Seq:<br># 朱一龙温柔的力量 [ 超话 ] # # 朱一龙并肩前行 #<br>#Yilong Zhu Gentle power [super topic]# #Yilong Zhu, move forward together# |
| PCGN U1:<br>『朱一龙 』甜有 100 种方式，吃糖，还有每天 99 次的想你 。<br>There is one hunderd ways of sweetness, have a candy and miss you 99 times a day. |
| PCGN U2:<br>#朱一龙温柔的力量 [ 超话 ] # #朱一龙 并肩前行 # 朱一龙 \| ZYL<br>#Yilong Zhu Gentle power [super topic]# #Yilong Zhu, move forward together# Yilong Zhu\| ZYL |
| PCGN U3:<br>『 朱一龙 』愿你一直如少年，干净纯粹心安， 看透不美好却相信美好<br>I hope that you are always young, with a clean and pure heart, always believing something beautiful |

Figure 2: Generated comments based on blog of different users. Since Seq2Seq model does not take user profile into consideration, it generates same comments for the same blog.

| **Blog** |
| --- |
| # 我的真朋友# 运用日剧和漫画的镜头切割，芭莎特别策划打造视觉大片，将三位主演的剧中人物关系呈现在视觉大片里， 让你在放映前先睹为快! Angelababy 发型/刘雪亮 Angelababy 化妆/春楠 邓伦妆发/李健成 朱一龙妆发/李鹏坤<br>#My true friend # Using the lens of Japanese TV dramas and comics, Bazaar specially plans to create visual blockbusters, and present the relationship among the three main characters in the photo, which will give you a sneak of the movie before its showing! Angelababy Hairstyle / Liu Xueliang Angelababy Makeup / Chun Nan Lun Deng makeup hair / Jiancheng Li Yilong Zhu makeup hair / Pengkun Li |
| **Comments** |
| Seq2Seq:<br># angelababy [ 超话 ] #<br># angelababy [super topic] # |
| PCGN U1:<br># 朱一龙[ 超话 ] # # 朱一 龙井然 # 期待井然哥哥<br>Yilong Zhu[super topic]# #朱一龙井然# Looking forward to Jingan brother |
| PCGN U2:<br>期待 期待<br>looking forward to |
| PCGN U3:<br>期待邓伦<br>looking forward to Lun Deng |

Figure 3: Generated comments based on blog of different users.
